# Supplementary material for: The Power of Learned Locally Linear Models for Nonlinear Policy Optimization
Source: arXiv:2305.09619 source file (2023-05-16)
Supplement: Supplementary file 1 [file appendix.tex]

%!TEX root = ../main.tex

\newpage

\section{Supplementary Proofs}\label{append:proofs}

%\matrixhoeffding*
